# Supplementary material for: SwinTrack: A Simple and Strong Baseline for Transformer Tracking
Source: arXiv:2112.00995 source file (2022-10-13)
Supplement: Supplementary file 1 [file precision_plot.tex]

% This file was created with tikzplotlib v0.10.1.
\begin{tikzpicture}

\definecolor{cyan}{RGB}{0,255,255}
\definecolor{darkgray176}{RGB}{176,176,176}
\definecolor{magenta}{RGB}{255,0,255}

\begin{axis}[
legend cell align={left},
legend style={fill opacity=1.0, draw opacity=1, text opacity=1, at={(0.97,0.03)}, anchor=south east},
tick align=outside,
tick pos=left,
title={Precision plot},
x grid style={darkgray176},
xlabel={Location error threshold [pixels]},
xmajorgrids,
xmin=0, xmax=50,
xtick style={color=black},
y grid style={darkgray176},
ylabel={Distance Precision [\%]},
ymajorgrids,
ymin=0, ymax=100,
ytick style={color=black}
]
\addplot [thick, gray]
table {%
0 0.262796401977539
1 2.92494678497314
2 10.190544128418
3 19.9362564086914
4 27.7649917602539
5 34.5488357543945
6 39.0803070068359
7 43.3819274902344
8 46.6925659179688
9 49.6027603149414
10 52.2570114135742
11 54.4609298706055
12 56.3484420776367
13 58.1590347290039
14 59.6615142822266
15 61.0391502380371
16 62.2786178588867
17 63.412712097168
18 64.4432754516602
19 65.3986053466797
20 66.3043060302734
21 67.0943756103516
22 67.8381958007812
23 68.5027008056641
24 69.1230239868164
25 69.7038269042969
26 70.2364120483398
27 70.7172164916992
28 71.1825637817383
29 71.6061248779297
30 72.0104827880859
31 72.4028854370117
32 72.7599487304688
33 73.0978164672852
34 73.4144897460938
35 73.7288436889648
36 74.0205841064453
37 74.3186111450195
38 74.6056289672852
39 74.8804397583008
40 75.1385040283203
41 75.3983688354492
42 75.6448211669922
43 75.8898162841797
44 76.1138153076172
45 76.331916809082
46 76.5346755981445
47 76.7312622070312
48 76.9156341552734
49 77.1044921875
50 77.2947845458984
};
\addlegendentry{TrDiMP [66.3]}
\addplot [thick, cyan]
table {%
0 0.0504663623869419
1 6.35006046295166
2 17.6777515411377
3 27.51123046875
4 35.1705627441406
5 41.1083030700684
6 45.8147506713867
7 49.6967582702637
8 52.8312377929688
9 55.4575309753418
10 57.713550567627
11 59.6219940185547
12 61.252628326416
13 62.6995315551758
14 63.9634971618652
15 65.0405883789062
16 65.9823913574219
17 66.8850479125977
18 67.6832656860352
19 68.3992691040039
20 69.0166091918945
21 69.5805282592773
22 70.0909881591797
23 70.5376739501953
24 70.92724609375
25 71.3039703369141
26 71.6530914306641
27 71.9626617431641
28 72.2531585693359
29 72.5363845825195
30 72.7947082519531
31 73.0490875244141
32 73.2917861938477
33 73.5275650024414
34 73.7428741455078
35 73.9558868408203
36 74.1648101806641
37 74.3626861572266
38 74.5630416870117
39 74.7482299804688
40 74.9167938232422
41 75.0783462524414
42 75.2441482543945
43 75.4030456542969
44 75.5633392333984
45 75.7098388671875
46 75.8620147705078
47 76.0291213989258
48 76.1782684326172
49 76.3012466430664
50 76.4280395507812
};
\addlegendentry{TransT [69.0]}
\addplot [thick, magenta]
table {%
0 0.0504663623869419
1 8.82082366943359
2 21.6383800506592
3 31.2220611572266
4 38.507209777832
5 44.0193634033203
6 48.4878005981445
7 52.1530570983887
8 55.1679916381836
9 57.7008743286133
10 59.8693313598633
11 61.6847267150879
12 63.2172889709473
13 64.5631484985352
14 65.7556457519531
15 66.8354949951172
16 67.7942886352539
17 68.6865234375
18 69.4827346801758
19 70.1895065307617
20 70.8372116088867
21 71.4245758056641
22 71.9685516357422
23 72.4641418457031
24 72.9245529174805
25 73.3448638916016
26 73.756721496582
27 74.1450805664062
28 74.5152206420898
29 74.8672561645508
30 75.1938400268555
31 75.5105285644531
32 75.8148727416992
33 76.0864944458008
34 76.3699798583984
35 76.6304931640625
36 76.8664627075195
37 77.1056671142578
38 77.3082580566406
39 77.5058670043945
40 77.7110137939453
41 77.9050598144531
42 78.0927810668945
43 78.2720947265625
44 78.4523620605469
45 78.6244049072266
46 78.8016357421875
47 78.9714889526367
48 79.127571105957
49 79.2715682983398
50 79.4226837158203
};
\addlegendentry{SwinTrack-T-224 [70.8]}
\addplot [thick, black]
table {%
0 0.264687269926071
1 2.66286325454712
2 10.2780637741089
3 22.2662029266357
4 32.0875625610352
5 40.306453704834
6 45.5220031738281
7 50.2590065002441
8 53.7944679260254
9 56.7636795043945
10 59.3387718200684
11 61.4541282653809
12 63.2197494506836
13 64.878547668457
14 66.2517166137695
15 67.5147247314453
16 68.6433563232422
17 69.7103118896484
18 70.6519622802734
19 71.5002212524414
20 72.2395172119141
21 72.8751068115234
22 73.4193725585938
23 73.9048309326172
24 74.3532180786133
25 74.7707824707031
26 75.1520767211914
27 75.4855575561523
28 75.8070373535156
29 76.0983047485352
30 76.3693008422852
31 76.6468734741211
32 76.8952102661133
33 77.1156463623047
34 77.3304214477539
35 77.5635528564453
36 77.7762603759766
37 78.005615234375
38 78.2254409790039
39 78.4276809692383
40 78.6147689819336
41 78.7892303466797
42 78.9567642211914
43 79.121940612793
44 79.2837829589844
45 79.4345550537109
46 79.5879745483398
47 79.735107421875
48 79.8767013549805
49 80.0132751464844
50 80.1515197753906
};
\addlegendentry{STARK [72.2]}
\addplot [thick, blue]
table {%
0 0.505607068538666
1 5.36885499954224
2 16.2277641296387
3 27.1090545654297
4 34.9986419677734
5 41.7345771789551
6 46.4616050720215
7 51.0711898803711
8 54.6231918334961
9 57.6373710632324
10 60.3525047302246
11 62.6116561889648
12 64.4953079223633
13 66.2497940063477
14 67.6984405517578
15 69.0177154541016
16 70.1415863037109
17 71.1519165039062
18 72.0068206787109
19 72.7753143310547
20 73.5076751708984
21 74.1445083618164
22 74.7381820678711
23 75.2673492431641
24 75.7610168457031
25 76.259391784668
26 76.704475402832
27 77.1144180297852
28 77.5067825317383
29 77.8565902709961
30 78.1669769287109
31 78.4766845703125
32 78.7707901000977
33 79.0440521240234
34 79.3026885986328
35 79.5458145141602
36 79.7714309692383
37 80.0000686645508
38 80.2222671508789
39 80.4377670288086
40 80.6393356323242
41 80.8413619995117
42 81.0181045532227
43 81.2052612304688
44 81.3865509033203
45 81.546989440918
46 81.7103118896484
47 81.8591690063477
48 82.0022811889648
49 82.1379089355469
50 82.2716445922852
};
\addlegendentry{ToMP [73.5]}
\addplot [thick, green]
table {%
0 0.304750382900238
1 3.23846530914307
2 12.5862970352173
3 26.6148262023926
4 37.6737747192383
5 46.376880645752
6 51.8484420776367
7 56.7283515930176
8 60.223503112793
9 63.0621147155762
10 65.4960861206055
11 67.4364929199219
12 69.0585098266602
13 70.5485000610352
14 71.7113876342773
15 72.7361907958984
16 73.6279449462891
17 74.4316482543945
18 75.1371002197266
19 75.7486801147461
20 76.3344039916992
21 76.8381195068359
22 77.33544921875
23 77.7434387207031
24 78.1199722290039
25 78.4653930664062
26 78.7747116088867
27 79.0489730834961
28 79.3204879760742
29 79.5672836303711
30 79.8155517578125
31 80.0505752563477
32 80.2650985717773
33 80.4735488891602
34 80.6727676391602
35 80.8591613769531
36 81.0416107177734
37 81.211784362793
38 81.3712310791016
39 81.5326538085938
40 81.6760635375977
41 81.8192443847656
42 81.9595108032227
43 82.1002044677734
44 82.2351379394531
45 82.3682479858398
46 82.4833831787109
47 82.5873260498047
48 82.6947708129883
49 82.8041076660156
50 82.9195098876953
};
\addlegendentry{MixFormer [76.3]}
\addplot [thick, red]
table {%
0 0.0504663623869419
1 11.8184518814087
2 28.1475982666016
3 39.6667289733887
4 47.7942314147949
5 53.6860885620117
6 58.1003837585449
7 61.6025276184082
8 64.4151992797852
9 66.6277313232422
10 68.3537902832031
11 69.7637023925781
12 70.930549621582
13 71.9451446533203
14 72.8109664916992
15 73.5948333740234
16 74.2950057983398
17 74.9093780517578
18 75.4595718383789
19 75.9770965576172
20 76.4579238891602
21 76.8763275146484
22 77.2583541870117
23 77.6085052490234
24 77.935188293457
25 78.2289581298828
26 78.5010604858398
27 78.7525863647461
28 78.9847564697266
29 79.2096710205078
30 79.4118957519531
31 79.6002960205078
32 79.7815246582031
33 79.9609222412109
34 80.1327056884766
35 80.3031997680664
36 80.45068359375
37 80.5997009277344
38 80.7397308349609
39 80.8952789306641
40 81.0318756103516
41 81.1686553955078
42 81.2992172241211
43 81.4214248657227
44 81.5451126098633
45 81.6689224243164
46 81.7865219116211
47 81.9021072387695
48 82.0111312866211
49 82.1211853027344
50 82.2361602783203
};
\addlegendentry{SwinTrack-B-384 [76.5]}
\end{axis}

\end{tikzpicture}
