# Supplementary material for: SwinTrack: A Simple and Strong Baseline for Transformer Tracking
Source: arXiv:2112.00995 source file (2022-10-13)
Supplement: Supplementary file 2 [file precision_plot.tex]

% This file was created with tikzplotlib v0.10.1.
\begin{tikzpicture}

\definecolor{darkgray176}{RGB}{176,176,176}

\begin{axis}[
legend cell align={left},
legend style={fill opacity=1.0, draw opacity=1, text opacity=1, at={(0.97,0.03)}, anchor=south east},
tick align=outside,
tick pos=left,
title={Precision plot},
x grid style={darkgray176},
xlabel={Location error threshold [pixels]},
xmajorgrids,
xmin=0, xmax=50,
xtick style={color=black},
y grid style={darkgray176},
ylabel={Distance Precision [\%]},
ymajorgrids,
ymin=0, ymax=100,
ytick style={color=black}
]
\addplot [thick, black]
table {%
0 0.0504663623869419
1 8.46163272857666
2 20.8333606719971
3 30.1140193939209
4 37.180606842041
5 42.6359939575195
6 47.0817680358887
7 50.8075790405273
8 53.9556846618652
9 56.5992660522461
10 58.8906402587891
11 60.8490180969238
12 62.5650177001953
13 64.0610122680664
14 65.3373031616211
15 66.500129699707
16 67.5050964355469
17 68.4029922485352
18 69.1713256835938
19 69.9066162109375
20 70.5755157470703
21 71.1993865966797
22 71.7446899414062
23 72.2436828613281
24 72.6890640258789
25 73.1140365600586
26 73.5050048828125
27 73.869010925293
28 74.235954284668
29 74.5569915771484
30 74.8698577880859
31 75.1739120483398
32 75.4675903320312
33 75.7525253295898
34 76.0183334350586
35 76.2531661987305
36 76.472282409668
37 76.6931762695312
38 76.9036407470703
39 77.1119537353516
40 77.3035202026367
41 77.4973220825195
42 77.6762542724609
43 77.8576583862305
44 78.0350570678711
45 78.2102203369141
46 78.366096496582
47 78.5194625854492
48 78.6722717285156
49 78.8311920166016
50 78.9822845458984
};
\addlegendentry{SwinTrack-T-224-NoMToken [70.6]}
\addplot [thick, blue]
table {%
0 0.0504663623869419
1 8.54149627685547
2 21.668550491333
3 31.3686428070068
4 38.7215690612793
5 44.4532356262207
6 49.0336990356445
7 52.8022994995117
8 55.944206237793
9 58.5594711303711
10 60.7948417663574
11 62.6697769165039
12 64.2466659545898
13 65.6322631835938
14 66.8576431274414
15 67.9185104370117
16 68.8499603271484
17 69.6802368164062
18 70.4302825927734
19 71.1034927368164
20 71.700325012207
21 72.2448043823242
22 72.743766784668
23 73.1937561035156
24 73.6177597045898
25 74.0081481933594
26 74.3532028198242
27 74.6963043212891
28 74.997688293457
29 75.2951583862305
30 75.5783309936523
31 75.8594589233398
32 76.1351623535156
33 76.3878860473633
34 76.6323776245117
35 76.861442565918
36 77.0885848999023
37 77.3006286621094
38 77.4937438964844
39 77.6705169677734
40 77.8608703613281
41 78.0410003662109
42 78.2137756347656
43 78.3741912841797
44 78.542724609375
45 78.7067108154297
46 78.8710556030273
47 79.0150604248047
48 79.1560974121094
49 79.2953186035156
50 79.4211502075195
};
\addlegendentry{SwinTrack-T-224-22k-NoMToken [71.7]}
\addplot [thick, green]
table {%
0 0.0504663623869419
1 10.7928762435913
2 26.0834579467773
3 36.6809387207031
4 44.0788803100586
5 49.5271339416504
6 53.6652221679688
7 56.9898300170898
8 59.7014617919922
9 61.8717193603516
10 63.6504783630371
11 65.1922607421875
12 66.4725799560547
13 67.5518341064453
14 68.4899444580078
15 69.3267593383789
16 70.0778732299805
17 70.754753112793
18 71.3657989501953
19 71.9274444580078
20 72.4528350830078
21 72.9573211669922
22 73.3919906616211
23 73.7910003662109
24 74.1562652587891
25 74.4700469970703
26 74.7722473144531
27 75.0556793212891
28 75.3276062011719
29 75.56787109375
30 75.7884826660156
31 75.9919128417969
32 76.1896438598633
33 76.3827438354492
34 76.5612030029297
35 76.7576599121094
36 76.9406585693359
37 77.1035614013672
38 77.2647705078125
39 77.4130859375
40 77.5576934814453
41 77.7002105712891
42 77.8431243896484
43 77.9792938232422
44 78.1228637695312
45 78.2722091674805
46 78.4214782714844
47 78.5647201538086
48 78.6961822509766
49 78.8268737792969
50 78.9407730102539
};
\addlegendentry{SwinTrack-B-384-1k-NoMToken [72.5]}
\addplot [thick, red]
table {%
0 0.0504663623869419
1 11.3507537841797
2 27.501615524292
3 38.8654556274414
4 46.7537078857422
5 52.5928611755371
6 57.0894165039062
7 60.5836219787598
8 63.3018035888672
9 65.4725646972656
10 67.2124557495117
11 68.6652221679688
12 69.8958129882812
13 70.9169082641602
14 71.788215637207
15 72.566650390625
16 73.2369613647461
17 73.8309860229492
18 74.3663482666016
19 74.8588943481445
20 75.326904296875
21 75.7556762695312
22 76.1479644775391
23 76.5143966674805
24 76.8414459228516
25 77.1409378051758
26 77.390983581543
27 77.6254043579102
28 77.8582305908203
29 78.0759735107422
30 78.2733535766602
31 78.4513931274414
32 78.6177368164062
33 78.7706298828125
34 78.9235687255859
35 79.0780944824219
36 79.2373123168945
37 79.3906860351562
38 79.5198516845703
39 79.6586990356445
40 79.7798461914062
41 79.890380859375
42 80.0062484741211
43 80.120002746582
44 80.234733581543
45 80.3514785766602
46 80.4606552124023
47 80.5631103515625
48 80.66796875
49 80.7707443237305
50 80.8708877563477
};
\addlegendentry{SwinTrack-B-384-NoMToken [75.3]}
\end{axis}

\end{tikzpicture}
