# Supplementary material for: SwinTrack: A Simple and Strong Baseline for Transformer Tracking
Source: arXiv:2112.00995 source file (2022-10-13)
Supplement: Supplementary file 3 [file success_plot.tex]

% This file was created with tikzplotlib v0.10.1.
\begin{tikzpicture}

\definecolor{darkgray176}{RGB}{176,176,176}

\begin{axis}[
legend cell align={left},
legend style={fill opacity=1.0, draw opacity=1, text opacity=1, at={(0.03,0.03)}, anchor=south west},
tick align=outside,
tick pos=left,
title={Success plot},
x grid style={darkgray176},
xlabel={Overlap threshold},
xmajorgrids,
xmin=0, xmax=1,
xtick style={color=black},
y grid style={darkgray176},
ylabel={Overlap Precision [\%]},
ymajorgrids,
ymin=0, ymax=100,
ytick style={color=black}
]
\addplot [thick, black]
table {%
0 85.3124008178711
0.0500000007450581 83.784065246582
0.100000001490116 82.8986511230469
0.150000005960464 82.199348449707
0.200000002980232 81.6311187744141
0.25 81.1087036132812
0.300000011920929 80.5525436401367
0.349999994039536 79.9055252075195
0.400000005960464 79.166862487793
0.449999988079071 78.3173751831055
0.5 77.1825637817383
0.550000011920929 75.8297119140625
0.600000023841858 74.2671813964844
0.649999976158142 72.1601104736328
0.699999988079071 69.3161926269531
0.75 65.2747192382812
0.800000011920929 59.0510787963867
0.850000023841858 49.2461814880371
0.899999976158142 33.1640968322754
0.949999988079071 10.2892179489136
1 0
};
\addlegendentry{SwinTrack-T-224-NoMToken [66.7]}
\addplot [thick, blue]
table {%
0 84.96630859375
0.0500000007450581 83.7192001342773
0.100000001490116 82.9853363037109
0.150000005960464 82.4537582397461
0.200000002980232 81.9464569091797
0.25 81.4738693237305
0.300000011920929 80.92919921875
0.349999994039536 80.2817611694336
0.400000005960464 79.5831527709961
0.449999988079071 78.8810424804688
0.5 77.9166107177734
0.550000011920929 76.7832794189453
0.600000023841858 75.3112106323242
0.649999976158142 73.3368682861328
0.699999988079071 70.6721343994141
0.75 66.8370895385742
0.800000011920929 60.5997505187988
0.850000023841858 50.6270942687988
0.899999976158142 33.9694671630859
0.949999988079071 10.2846155166626
1 0
};
\addlegendentry{SwinTrack-T-224-22k-NoMToken [67.3]}
\addplot [thick, green]
table {%
0 84.3527450561523
0.0500000007450581 83.2119598388672
0.100000001490116 82.3309097290039
0.150000005960464 81.7581481933594
0.200000002980232 81.2836380004883
0.25 80.7989501953125
0.300000011920929 80.314079284668
0.349999994039536 79.7022171020508
0.400000005960464 79.0056762695312
0.449999988079071 78.1660842895508
0.5 77.3199234008789
0.550000011920929 76.2883834838867
0.600000023841858 74.902946472168
0.649999976158142 73.1230239868164
0.699999988079071 70.7664794921875
0.75 67.5476837158203
0.800000011920929 62.7710151672363
0.850000023841858 55.3399696350098
0.899999976158142 41.8096809387207
0.949999988079071 17.7590408325195
1 0
};
\addlegendentry{SwinTrack-B-384-1k-NoMToken [68.0]}
\addplot [thick, red]
table {%
0 85.850227355957
0.0500000007450581 84.7379379272461
0.100000001490116 84.1397018432617
0.150000005960464 83.7286987304688
0.200000002980232 83.3811416625977
0.25 82.9725036621094
0.300000011920929 82.5358123779297
0.349999994039536 81.955322265625
0.400000005960464 81.282958984375
0.449999988079071 80.5210647583008
0.5 79.7132339477539
0.550000011920929 78.7315979003906
0.600000023841858 77.4594192504883
0.649999976158142 75.8076171875
0.699999988079071 73.6182556152344
0.75 70.5351638793945
0.800000011920929 65.7851028442383
0.850000023841858 57.7718811035156
0.899999976158142 43.9315452575684
0.949999988079071 19.8706531524658
1 0
};
\addlegendentry{SwinTrack-B-384-NoMToken [70.2]}
\end{axis}

\end{tikzpicture}
