# Supplementary material for: SwinTrack: A Simple and Strong Baseline for Transformer Tracking
Source: arXiv:2112.00995 source file (2022-10-13)
Supplement: Supplementary file 4 [file success_plot.tex]

% This file was created with tikzplotlib v0.10.1.
\begin{tikzpicture}

\definecolor{cyan}{RGB}{0,255,255}
\definecolor{darkgray176}{RGB}{176,176,176}
\definecolor{magenta}{RGB}{255,0,255}

\begin{axis}[
legend cell align={left},
legend style={fill opacity=1.0, draw opacity=1, text opacity=1, at={(0.03,0.03)}, anchor=south west},
tick align=outside,
tick pos=left,
title={Success plot},
x grid style={darkgray176},
xlabel={Overlap threshold},
xmajorgrids,
xmin=0, xmax=1,
xtick style={color=black},
y grid style={darkgray176},
ylabel={Overlap Precision [\%]},
ymajorgrids,
ymin=0, ymax=100,
ytick style={color=black}
]
\addplot [thick, gray]
table {%
0 85.3563690185547
0.0500000007450581 84.338981628418
0.100000001490116 83.6399612426758
0.150000005960464 83.0258865356445
0.200000002980232 82.3551254272461
0.25 81.5988235473633
0.300000011920929 80.6928863525391
0.349999994039536 79.5506744384766
0.400000005960464 78.3844985961914
0.449999988079071 77.0281066894531
0.5 75.3514938354492
0.550000011920929 73.4308624267578
0.600000023841858 71.1521530151367
0.649999976158142 68.1578063964844
0.699999988079071 64.17919921875
0.75 58.5912780761719
0.800000011920929 50.4710807800293
0.850000023841858 38.5650825500488
0.899999976158142 21.2922058105469
0.949999988079071 3.87033033370972
1 0
};
\addlegendentry{TrDiMP [63.9]}
\addplot [thick, cyan]
table {%
0 82.1811447143555
0.0500000007450581 81.130126953125
0.100000001490116 80.4880905151367
0.150000005960464 79.9483261108398
0.200000002980232 79.524528503418
0.25 79.0952606201172
0.300000011920929 78.5835418701172
0.349999994039536 77.9458847045898
0.400000005960464 77.0856170654297
0.449999988079071 76.3620223999023
0.5 75.2638168334961
0.550000011920929 74.1415328979492
0.600000023841858 72.6995391845703
0.649999976158142 70.7366256713867
0.699999988079071 68.0166931152344
0.75 64.0507049560547
0.800000011920929 58.0414237976074
0.850000023841858 48.0121994018555
0.899999976158142 31.1894454956055
0.949999988079071 7.37785196304321
1 0
};
\addlegendentry{TransT [64.9]}
\addplot [thick, magenta]
table {%
0 86.5059585571289
0.0500000007450581 85.4760131835938
0.100000001490116 84.6729583740234
0.150000005960464 84.0289077758789
0.200000002980232 83.5075607299805
0.25 82.9430541992188
0.300000011920929 82.3839340209961
0.349999994039536 81.7521133422852
0.400000005960464 80.8750228881836
0.449999988079071 80.0048522949219
0.5 78.9352111816406
0.550000011920929 77.7029876708984
0.600000023841858 76.1019973754883
0.649999976158142 73.7927780151367
0.699999988079071 70.3733291625977
0.75 65.2167816162109
0.800000011920929 57.0196075439453
0.850000023841858 44.9836959838867
0.899999976158142 26.5942611694336
0.949999988079071 5.85685920715332
1 0
};
\addlegendentry{STARK [67.1]}
\addplot [thick, black]
table {%
0 85.5778732299805
0.0500000007450581 84.1035537719727
0.100000001490116 83.3299713134766
0.150000005960464 82.7461700439453
0.200000002980232 82.2377166748047
0.25 81.6727294921875
0.300000011920929 81.1188430786133
0.349999994039536 80.4158172607422
0.400000005960464 79.6402816772461
0.449999988079071 78.8200378417969
0.5 77.7748641967773
0.550000011920929 76.5463027954102
0.600000023841858 75.0328216552734
0.649999976158142 72.9672393798828
0.699999988079071 70.0464553833008
0.75 65.843864440918
0.800000011920929 59.4688186645508
0.850000023841858 49.6399803161621
0.899999976158142 33.6708564758301
0.949999988079071 10.8771266937256
1 0
};
\addlegendentry{SwinTrack-T-224 [67.2]}
\addplot [thick, blue]
table {%
0 87.6947326660156
0.0500000007450581 86.7127380371094
0.100000001490116 86.1569366455078
0.150000005960464 85.6223678588867
0.200000002980232 85.134162902832
0.25 84.6478958129883
0.300000011920929 84.1479339599609
0.349999994039536 83.5117721557617
0.400000005960464 82.6738510131836
0.449999988079071 81.8229904174805
0.5 80.7913818359375
0.550000011920929 79.4765777587891
0.600000023841858 77.7239761352539
0.649999976158142 75.3065414428711
0.699999988079071 71.794792175293
0.75 66.445671081543
0.800000011920929 58.2587738037109
0.850000023841858 45.7767219543457
0.899999976158142 27.6395320892334
0.949999988079071 7.11588954925537
1 0
};
\addlegendentry{ToMP [68.5]}
\addplot [thick, green]
table {%
0 87.9642944335938
0.0500000007450581 87.2290115356445
0.100000001490116 86.7096862792969
0.150000005960464 86.2598419189453
0.200000002980232 85.8123626708984
0.25 85.3485641479492
0.300000011920929 84.8339080810547
0.349999994039536 84.1455841064453
0.400000005960464 83.4091491699219
0.449999988079071 82.536491394043
0.5 81.5589141845703
0.550000011920929 80.459098815918
0.600000023841858 79.0383453369141
0.649999976158142 76.987548828125
0.699999988079071 73.9069366455078
0.75 69.3097763061523
0.800000011920929 62.1433563232422
0.850000023841858 51.0754776000977
0.899999976158142 33.3884429931641
0.949999988079071 8.84209823608398
1 0
};
\addlegendentry{MixFormer [70.0]}
\addplot [thick, red]
table {%
0 87.1718978881836
0.0500000007450581 86.1381683349609
0.100000001490116 85.4462280273438
0.150000005960464 84.9568328857422
0.200000002980232 84.5217132568359
0.25 84.090202331543
0.300000011920929 83.6422119140625
0.349999994039536 83.1625366210938
0.400000005960464 82.4673690795898
0.449999988079071 81.7340850830078
0.5 80.963996887207
0.550000011920929 79.9329605102539
0.600000023841858 78.6637268066406
0.649999976158142 77.0235595703125
0.699999988079071 74.7673721313477
0.75 71.6431579589844
0.800000011920929 66.8184432983398
0.850000023841858 58.8123397827148
0.899999976158142 44.7114028930664
0.949999988079071 20.9500827789307
1 0
};
\addlegendentry{SwinTrack-B-384 [71.3]}
\end{axis}

\end{tikzpicture}
